# Supplementary material for: Quantum Storage of Frequency-Multiplexed Photons Exhibiting Nonclassical Correlations with Telecom C-Band Photons
Source: arXiv:2511.16977 source file (2025-11-21)
Supplement: Supplementary file 1 [file arXiv_tateishi_supplementary.pdf]

# Supplementary Information for "Quantum Storage of Frequency-Multiplexed Photons Exhibiting Nonclassical Correlations with Telecom C-Band Photons"

Hiroki Tateishi,[1,*] Daisuke Yoshida,[2,3] Tomoki Tsuno,[1,3]
Takuto Nihashi,[1] Ryoma Komatsudaira,[1] Daisuke Akamatsu,[1]
Feng-Lei Hong,[1,2] Koji Nagano,[2,3] and Tomoyuki Horikiri[1,2,3,†]

[1]*Department of Physics, Yokohama National University,*
*79-5 Tokiwadai, Hodogaya-ku, Yokohama 240-8501,*
[2]*IMS, Yokohama National University,*
*79-5 Tokiwadai, Hodogaya-ku, Yokohama 240-8501,*
[3]*LQUOM, Inc.*

[*] tateishi-hiroki-tn@ynu.jp
[†] horikiri-tomoyuki-bh@ynu.ac.jp

## A. Preparation of a Frequency-Multiplexed Atomic Frequency Comb (AFC)

We prepared frequency-multiplexed atomic frequency combs (AFCs) on the $^3H_4 \leftrightarrow {}^1D_2$ transition of praseodymium-doped yttrium orthosilicate (Pr:YSO) at $\sim 605.98$ nm. The inhomogeneous broadening of this transition in Pr:YSO is $\sim 10$ GHz, which in principle allows many independent frequency modes. The hyperfine structure of Pr:YSO, however, imposes two practical constraints: (i) within each frequency mode the usable AFC bandwidth is limited to only a few megahertz, and (ii) independence between neighboring modes requires a spectral spacing of $\sim 100$ MHz in Pr:YSO [1]. In this work we chose a mode spacing of 123 MHz to match the cavity free spectral range (FSR).

Within one frequency mode, we formed a 4.6 MHz-wide comb with 920 kHz tooth spacing by modulating the pump via an acousto-optic modulator (AOM). This yields a regularly spaced sequence of absorption teeth over the mode bandwidth.

To prepare multiple frequency modes simultaneously, the pump laser was sent through a single electro-optic phase modulator (EOM) driven by a multi-tone waveform synthesized by an arbitrary waveform generator (AWG). The applied RF tones at 123 MHz, 369.01 MHz, and 1107.015 MHz generated optical sidebands that addressed distinct frequency modes with a mode-to-mode spacing of 123 MHz, equal to the cavity free spectral range (FSR). The three RF frequencies were chosen close to 1×, 3×, and 9× the FSR, with small intentional detunings to reduce overlap and interference between sidebands generated by different tones. The amplitudes of the individual RF components were adjusted to obtain the pump spectra shown in Fig. S1(a)–(d).

After preparing the AFCs, we characterized them by scanning a weak probe laser. The probe laser was independent of the preparation beam, and its frequency was swept with a slow triangular waveform. Because the sweep was not perfectly linear in frequency, the time axis of the raw transmission traces did not map linearly to optical frequency. We therefore calibrated the horizontal axis using the known center frequencies of the prepared AFC modes, which fixes their relative spacings and positions. The sweep direction was not recorded, so the sign of the relative-frequency axis in the plots is arbitrary.

Figure S2 shows AFCs prepared with pump spectra designed to realize the target spectra in Figs. S1(a)–(d). AFCs were created in more modes than intended: for targets of 3, 9, 27, and 63 modes, the measured AFCs formed in approximately 5, 15, 45, and 83 modes,

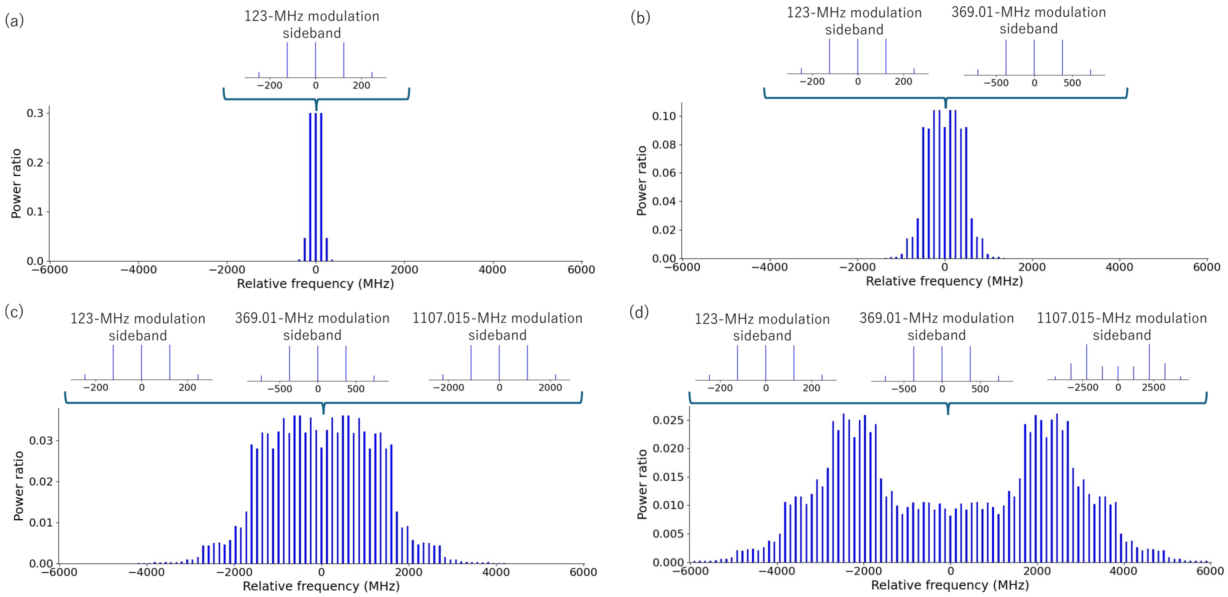


FIG. S1. **Target pump spectra.** In this experiment we created frequency-multiplexed AFCs using four sideband configurations. (a)–(d) show the target spectra. For each frequency mode, the power within a $\pm 1$ MHz window around the mode center is summed. **(a)** Target spectrum with 3 modes. **(b)** Target spectrum with 9 modes. **(c)** Target spectrum with 27 modes. **(d)** Target spectrum with 63 modes. The applied RF tones were: (a) 123 MHz; (b) 123 and 369.01 MHz; (c,d) 123, 369.01, and 1107.015 MHz.

respectively. We attribute this excess number of AFC modes to weak higher-order phase-modulation sidebands.

## B. Noise reduction system

In Fig. 3(a) of the main text, the noise floor is lower within a limited time window around the time when a photon retrieved from the memory is expected to be detected. This reduction of the noise floor arises from an active noise-reduction scheme: after the idler photon is detected, AOM shutter 3 is closed to block unwanted light. A schematic of this noise-reduction behavior is shown in Fig. S3.

During the photon-measurement sequence, if no idler heralding occurs, the AOM shutters 3 and 4 remain open, as shown in Fig. S3(a). In this condition the single-photon counting module (SPCM) detects the desired photons but may also detect background pho-

tons, mainly originating from the PPS path in the setup. When an idler photon is detected by the superconducting single-photon detector (SSPD), a corresponding signal photon is expected to be stored in the AFC and later retrieved. Using the SSPD output as a trigger, we temporarily close AOM 3 during the signal-detection window so that unwanted photons are suppressed while the retrieved signal is measured, as schematized in Fig. S3(b). This gating leads to the reduced noise level observed around the signal-retrieval timing in Fig. 3(a).

The AOMs are driven at 80 MHz. To gate shutter 3, we insert an RF switch (ZYSWA-2-50DR+, Mini-Circuits) in the RF line between the signal generator (SDG2122X, Siglent) and the AOM (AOMO3080-125, G&H). The RF switch is controlled by a digital delay/pulse generator (DG535, Stanford Research Systems) that is triggered by the SSPD output. Upon an idler click, the pulse generator applies a programmed blanking window of about 800 ns to AOM 3, thereby keeping unwanted background light blocked during the retrieved-signal detection window.

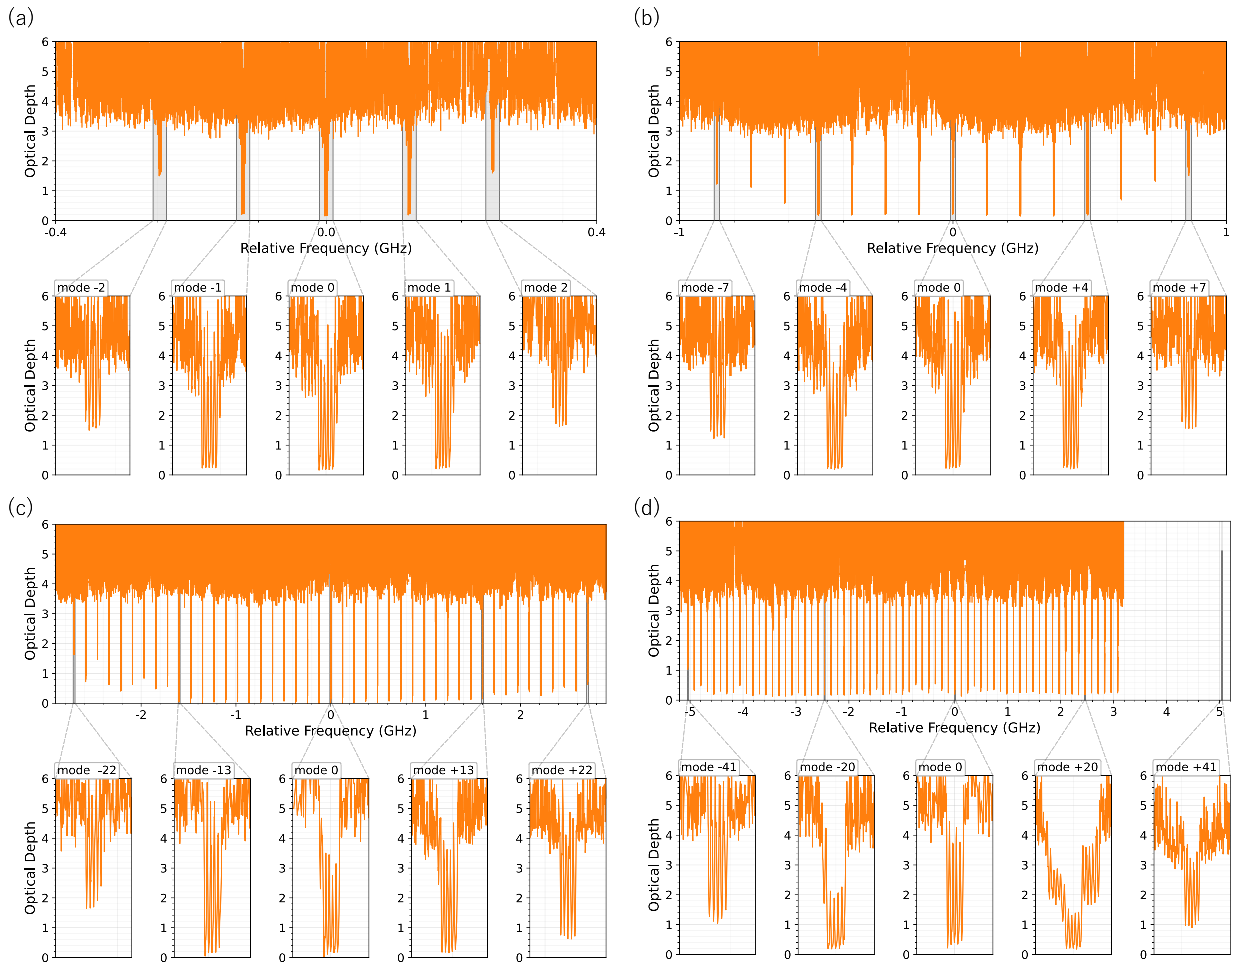


FIG. S2. **AFC spectra.** We created frequency-multiplexed AFCs using four sideband configurations. Panels (a)–(d) correspond to target settings of 3, 9, 27, and 63 modes and show the measured AFC spectra, which also include modes that formed outside the targets. **(a)** target: 3 modes. **(b)** target: 9 modes. **(c)** target: 27 modes. **(d)** target: 63 modes. In the measurements, the AFCs formed in more modes than targeted. The applied RF tones were: (a) 123 MHz, (b) 123 and 369.01 MHz, (c,d) 123, 369.01, and 1107.015 MHz. Probe spectra were taken with a probe laser separate from the preparation beam. Because the piezo-driven triangular scan is not perfectly linear, the frequency axis was calibrated to the AFC mode centers. The sign of the relative-frequency axis is arbitrary and carries no physical meaning, because the sweep direction was not enforced or tagged in this experiment.

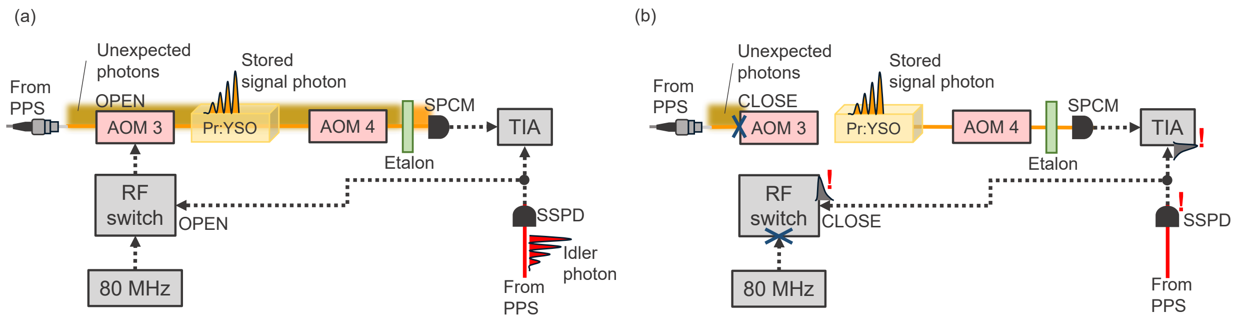


FIG. S3. (a) Photon-measurement sequence without herald. (b) Herald-gated mode.

## SUPPLEMENTARY REFERENCES

[1] Antonio Ortu, Jelena V. Rakonjac, Adrian Holzäpfel, Alessandro Seri, Samuele Grandi, Margherita Mazzera, Hugues de Riedmatten, and Mikael Afzelius, "Multimode capacity of atomic-frequency comb quantum memories," (2022).
